# Supplementary material for: Fresh Content Needs More Attention: Multi-funnel Fresh Content Recommendation
Source: arXiv:2306.01720 source file (2023-06-02)
Supplement: Supplementary file 1 [file Appendix.tex]

\section{Appendix}
\subsection{Datasets Details}
\label{sec:preprocess}

\smallskip
\noindent\textbf{Amazon.}
